# Supplementary material for: Parameter Space Noise for Exploration
Source: arXiv:1706.01905 source file (2018-01-31)
Supplement: Supplementary file 1 [file supplementary.tex]

\documentclass{article}

% if you need to pass options to natbib, use, e.g.:
% \PassOptionsToPackage{numbers, compress}{natbib}
% before loading nips_2017
%
% to avoid loading the natbib package, add option nonatbib:
% \usepackage[nonatbib]{nips_2017}

\usepackage{nips_2017}

% to compile a camera-ready version, add the [final] option, e.g.:
%\usepackage[final]{nips_2017}

\usepackage[utf8]{inputenc} % allow utf-8 input
\usepackage[T1]{fontenc}    % use 8-bit T1 fonts
\usepackage{hyperref}       % hyperlinks
\usepackage{url}            % simple URL typesetting
\usepackage{booktabs}       % professional-quality tables
\usepackage{amsfonts}       % blackboard math symbols
\usepackage{nicefrac}       % compact symbols for 1/2, etc.
\usepackage{microtype}      % microtypography

% Additional macros and packages.
\usepackage{amsmath}
\usepackage{amsfonts}
\usepackage{amssymb}
\usepackage{bbm}
\usepackage[inline]{enumitem}
\usepackage{tikz}
\usepackage{mathtools}
\usepackage{subfigure}


\renewcommand{\bibsection}{\subsection*{References}}

\DeclarePairedDelimiterX{\infdivx}[2]{(}{)}{%
  #1\;\delimsize\|\;#2%
}
\newcommand{\kl}{D_{\text{KL}}\infdivx}

\usepackage{bm}
\usepackage{xcolor}
\newcommand{\todo}[1]{\textcolor{red}{[TODO: #1]}}
\renewcommand{\vec}[1]{\boldsymbol{#1}}
\newcommand{\norm}[1]{\left\lVert#1\right\rVert}

\renewcommand{\S}{\mathcal{S}}
\renewcommand{\O}{\mathcal{O}}
\newcommand{\G}{\mathcal{G}}
\newcommand{\A}{\mathcal{A}}
\newcommand{\N}{\mathcal{N}}
\renewcommand{\L}{\mathcal{L}}
\newcommand{\R}{\mathbb{R}}
\newcommand{\E}{\mathbb{E}}
\newcommand{\1}{\mathbbm{1}}

\title{Parameter Space Noise for Exploration: Supplementary Material}
%%rein: Parameter Noise in Reinforcement Learning

% The \author macro works with any number of authors. There are two
% commands used to separate the names and addresses of multiple
% authors: \And and \AND.
%
% Using \And between authors leaves it to LaTeX to determine where to
% break the lines. Using \AND forces a line break at that point. So,
% if LaTeX puts 3 of 4 authors names on the first line, and the last
% on the second line, try using \AND instead of \And before the third
% author name.

% TODO: fix authors
\author{
  Matthias Plappert\thanks{Work done while interning at OpenAI.}\phantom{\footnotesize 1}\textsuperscript{,}\thanks{Correspondence to \texttt{matthiasplappert@me.com}.} \\
  Karlsruhe Institute of Technology \\
  \And
  Rein Houthooft \\
  OpenAI \\
  \And
  Prafulla Dhariwal \\
  OpenAI \\
  \And
  Marcin Andrychowicz \\
  OpenAI \\
  \And
  Pieter Abbeel \\
  UC Berkeley, OpenAI \\
}

\begin{document}

\maketitle

\appendix

\input{appendix}
\end{document}
